# Supplementary material for: Non-Monotonic Snapshot Isolation
Source: arXiv:1306.3906 source file (2013-06-17)
Supplement: Supplementary file 1 [file correctness_jessy.tex]

\section{Correctness of \jessy}
\labappendix{jessy}

In this section, we sketch a correctness proof of \jessy.
First, we establish  that \jessy generates \WSI histories in \refprop{cj:1}.
Then, \refprop{cj:2} shows that read-only transactions are wait-free, 
\refprop{cj:3} proves that updates are obstruction-free.
Finally, we show that \jessy satisfies a non-trivial progress condition in \refprop{cj:4}.

\subsection{Safety}
\labappendix{jessy:safety}

\begin{proposition}
  \labprop{cj:1}
  Every history admissible  by \jessy belongs to \WSI.
\end{proposition}

\begin{IEEEproof}  
  First of all, we observe that in \jessy transactions always reads
  from committed transactions (\refline{em:11} in \refalg{execution}).
  As a consequence, \jessy ensures \ACA.

  Consider now that a transaction $T_i$ read versions $x_l$ and $y_j$ of objects $x$ and $y$
  during some execution of \jessy.
  The two objects where read sequentially; 
  let us say $x$ before $y$.
  According to the code of the execution module,
  there exists a process $p$ replicating $y$ such 
  $p$ executes \reflines{em:2}{em:5} in \refalg{execution}.
  It follows that $\mvvOf{w_l(x_l)}[x] \geq \mvvOf{r_i(y_j)}[x]$ holds.
  Since $\mvvOf{r_i(x_l)}$ equals $\mvvOf{w_l(x_l)}$,
  we know that $\mvvOf{r_i(x_l)}[x] \geq \mvvOf{r_i(y_j)}[x]$ holds.
  Similarly, we deduce that $\mvvOf{r_i(y_j)}[y] \geq \mvvOf{r_i(x_l)}[y]$ holds.
  \reftheo{protocol:1} tells us that in such a case $T_i$ has read a consistent snapshot.

  It remains to show that that the histories generated by \jessy are write-conflict free.
  To this goal, we consider two independent write-conflicting transactions $T_i$ and $T_j$,
  and we assume for the sake of contradiction that they both commit.
  We note $p_i$ (resp. $p_j$) the coordinator of $T_i$ (resp. $T_j$).
  Since $T_i$ and $T_j$ write-conflict, 
  there exists some object $x$ in $\writeSetOf{T_i} \inter \writeSetOf{T_j}$.
  One can show, 
  using the preconditions of \dbDoCertify{},
  the monotonicity of variable \dbCertifyQueue,
  and the properties of atomic multicast, 
  that
  (F1) for any two replicas $p$ and $q$ of $x$, 
  denoting $\dbCommitted_p$ (resp. $\dbCommitted_q$) the set $\{ T_j \in \dbCommitted: x \in \writeSetOf{T_j} \}$,
  at the time $p$ (resp. $q$) executes $\dbVoteOutcome{T_i}$, 
  it is true that $\dbCommitted_p$ equals $\dbCommitted_q$.
  According to \refline{tp:9} of \refalg{termination} and the definition of function \dbVoteOutcome{},
  $p_i$ (respectively $p_j$) received a positive \voteMsg message 
  from some process $q_i$ (resp. $q_j$) replicating $x$.
  Observe that $T_i$ (resp. $T_j$) is in variable \dbCertifyQueue at process $q_i$ (resp. $q_j$)
  before this process sends its \voteMsg message.
  It follows that either (1) at the time $q_i$ sends its \voteMsg message, $T_j <_{\dbCertifyQueue} T_i$ holds,
  or (2) at the time $q_j$ sends its \voteMsg message, $T_i <_{\dbCertifyQueue} T_j$ holds.
  Assume that case (1) holds (the reasoning for case (2) is symmetrical).
  From the precondition at \refline{tp:6} in \refalg{termination} 
  we know that process $q_i$ must wait that $T_j$ is decided before casting a vote for $T_i$.
  From fact F1 above, we easily deduce that $T_j$ is committed at process $q_i$.
  Hence, \dbCertify{T_i} returns \false at process $q_i$; a contradiction.
\end{IEEEproof}

\subsection{Liveness}
\labappendix{jessy:liveness}

\begin{lemma}
  \lablem{cj:1}
  For every transaction $T_i$,
  if $T_i$ is submitted at \coordOf{T_i} and \coordOf{T_i} is correct,
  $T_i$ eventually terminates at every correct process in $\replicaSetOf{T_i} \union \coordOf{T_i}$.
\end{lemma}

\begin{IEEEproof}
  According to the termination, validity and uniform agreement properties
  of atomic multicast, transaction $T_i$ is delivered 
  at every correct process in \wreplicaSetOf{T_i}.
  It is then enqueued in variable \dbCertifyQueue (\reflines{tp:3}{tp:4} in \refalg{termination}).

  Because \dbCertifyQueue is FIFO, 
  processes dequeue transactions in the order they deliver them (\reflines{tp:5}{tp:6}).
  The uniform prefix order and acyclicity properties of genuine atomic multicast ensure
  that no two processes in the system wait for a vote from each other.
  It follows that every correct replicas in \wreplicaSetOf{T_i} eventually dequeue $T_i$, and send
  the outcome of function \dbCertify{T_i} to other replicas in $\wreplicaSetOf{T_i} \union \coordOf{T_i}$ (\reflines{tp:7}{tp:8b}).

  Since there exists at least one correct replica for each object modified by $T_i$
  eventually every correct process in $\wreplicaSetOf{T_i} \union \coordOf{T_i}$ collects enough votes to decide upon the outcome of $T_i$
  (definition of predicate \dbVoteOutcome{T_i}).  
\end{IEEEproof}

\begin{lemma}
  \lablem{cj:2}
  For every transaction $T_i$,
  if \coordOf{T_i} executes $T_i$ and \coordOf{T_i} is correct,
  then eventually $T_i$ is submitted to the termination protocol at \coordOf{T_i}.
\end{lemma}

\begin{IEEEproof}
  Transaction $T_i$ executes all its write operation locally at \coordOf{T_i}.
  Upon receiving a read request for an object $x$, if $x$ was modified previously
  by $T_i$, the corresponding value is returned.
  Otherwise, the transaction send a \readResolveMsg request to \replicaSetOf{x}. 
  Thus to prove the lemma, 
  we have to show that eventually one of the replicas returns a value of $x$ back to the coordinator.

  According to the model, there exists one correct process that replicates object $x$.
  In what follows, we name it $p$.
  Upon receiving the \readResolveMsg message from \coordOf{T_i},
  process $p$ tries to return a value of $x$ such that preconditions at \reflines{em:2}{em:4} hold. 

  By contradiction, assume that replica $p$ never finds such a version.
  This means that the following predicate is always true:
  \begin{displaymath}
    \begin{array}{l@{~}l}
      \forall y \in \readSetOf{T_i}, & \forall (x,v,l) \in \dbDatabase: \\  
      & \mvvOf{w_l(x_l)}[x] < \mvvOf{r_i(y_j)}[x] \\
      & \vee~ \mvvOf{w_l(x_l)}[y] > \mvvOf{r_i(y_j)}[y]
    \end{array}
  \end{displaymath}
  We consider two cases:
  \begin{enumerate}
  \item $\mvvOf{w_l(x_l)}[x] < \mvvOf{r_i(y_j)}[x]$ forever holds.\\
    According to the definition of function \mvvOfFunction,
    there exists a version $x_{k \neq 0}$ of object $x$ written by some
    transaction $T_k$ upon which transaction $T_i$ depends,
    and such that $\mvvOf{w_k(x_k)}[x]=\mvvOf{r_i(y_j)}[x]$.
    Because transaction $T_k$ committed at some site, 
    \reflem{cj:1} and \refprop{cj:1} tell us 
    that eventually $T_k$ commits at process $p$.
    Contradiction.
  \item $\mvvOf{w_l(x_l)}[y] > \mvvOf{r_i(y_j)}[y]$ forever holds.\\
      This case is symmetric to the case above, and thus omitted.
    \end{enumerate}
\end{IEEEproof}

\begin{proposition}
  \labprop{cj:2}
  Read-only transactions are wait-free.
\end{proposition}

\begin{IEEEproof}
  Consider some read-only transaction $T_i$ and assume that \coordOf{T_i} is correct,
  \reflem{cj:2} tells us that $T_i$ is eventually submitted at \coordOf{T_i}

  According to the definition of predicate \dbVoteOutcomeFunction, \dbVoteOutcome{T_i} always equals true. 
  Hence, the precondition at \refline{tp:9} in \refalg{termination} is always true,
  whereas precondition at \refline{tp:13} is always false.
  It follows that $T_i$  eventually commits.
\end{IEEEproof}

\begin{proposition}
  \labprop{cj:3}
  Updates transactions are obstruction-free.
\end{proposition}

\begin{IEEEproof}
  Consider some update transaction $T_i$ such that  \coordOf{T_i} is correct.
  From the conjunction of Lemmata~\ref{lem:cj:1}~and~\ref{lem:cj:2},
  transaction $T_i$ eventually terminates.
  
  Then, assume that at the time $T_i$ starts its execution,
  every transaction write-conflicting with $T_i$ has terminated.
  This implies that $T_i$ depends on every write-conflicting transactions.
  Thus, the outcome of $\dbCertify{T_i}$ always equals true.
  Hence, transaction $T_i$ eventually commits.
\end{IEEEproof}

\subsection{Non-triviality}
\labappendix{jessy:ntsi}

In this section, we show that \jessy implements the following progress condition:
\begin{itemize}

\item \textbf{Non-trivial \WSI.}
  Consider an admissible history $h$ such that 
  a transaction $T_i$ is pending in $h$, and the next operation of $T_i$ is a read on some object $x$.
  Note $x_j$ the latest committed version of $x$ in $h$.
  Let $\run$ be an execution with $\mathfrak{F}(\run)=h$.
  If there is no concurrent conflicting transaction to $T_i$ in $h$, and history $h'=h.r_i(x_j)$ is in $\WSI$,
  then there exists an execution $\run'$ extending $\run$ such that $\mathfrak{F}(\run')=h'$.
\end{itemize}

To this goal, 
we consider that (P1) when a process resolves a remote read request over some object $x$ at \reflines{em:3}{em:4},
it always returns the greatest version of $x$ (in the sense of function \mvvOfFunction) stored in variable \dbDatabase.
Since Jessy produces histories satisfying \WCF, there a single such version.

\begin{proposition}
  \labprop{cj:4}
  Consider an admissible history $h$ containing a pending transaction $T_i$
  such that
  the next operation of $T_i$ is a read over some object $x$.
  Note $x_j$ the latest committed version of $x$ in $h$.
  If history $h'=h.r_i(x_j)$ belongs to \WSI then history $h'$ is admissible.
\end{proposition}

\begin{IEEEproof}
  Consider a replica $p$ of $x$ storing version $x_j$,
  and assume from now that process $p$ always answers first to a
  remote read request from \coordOf{T_i} over $x$.
  Since history $h.r_i(x_j)$ is in $\WSI$, it belongs to $\CONS$. 
  As a consequence, $T_i$ reads a consistent snapshot in $h.r_j(x_i)$.
  According to \refprop{cv:3}, it follows that both 
  $\mvvOf{r_i(x_j)}[x] \geq \mvvOf{r_i(y_k)}[x]$
  and $\mvvOf{r_i(x_j)}[y] \leq \mvvOf{r_i(y_k)}[y]$ hold.
  According to the preconditions of operation $\dbReadResolve{x,T_i}$
  and the property P1 above, process $p$ returns version $x_j$ to \coordOf{T_i}.
\end{IEEEproof}
