# Supplementary material for: Non-Monotonic Snapshot Isolation
Source: arXiv:1306.3906 source file (2013-06-17)
Supplement: Supplementary file 2 [file phenomena.tex]

\section{Phenomena characterization of \WSI}
\labappendix{phenomena}
 
\begin{proposition}
  \labprop{phenomena:1}
  History $h$ does not observe phenomenon G-single if $h$ belongs to $\CONS
  \inter \WCF$
\end{proposition}

\begin{IEEEproof}
  By contradiction, assume a history $h$ such that $h \in \CONS \cap
   \WCF$ and phenomenon G-single is observed.

  Therefore, there exists a directed cycle with exactly one anti-dependency edge
  in DSG(h). 

  Case a) There is a ww edge in the cycle between $T_i$ and $T_j$ while there is
  not a wr edge between them. Thus, $T_i \cc T_j \wedge ws(T_i) \cap
  ws(T_j) \neq \varnothing \Rightarrow h \notin \WCF$. A contradiction to the assumption.

  Case b) There is not any ww edge in the cycle. Therefore, the cycle comprises of
  several wr edges and one rw edge from $T_i$ to $T_j$. Since there is a path
  with only wr edges from $T_j$ to $T_i$, we have $T_i \depend T_j$. Moreover, rw
  edge enforce that $\exists x_k : r_i(x_k) \in h \wedge w_j(x_j) \in h : x_j \gg
  x_k$. Thus, $h \notin \CONS$. A contradiction to the assumption. 
\end{IEEEproof}

\begin{proposition}
  \labprop{phenomena:2}
  History $h$ does not observe phenomenon G-1 if $h$ is in  $\ACA \inter \WCF$
\end{proposition}

\begin{IEEEproof}
  In order to prove the proposition, we prove that non of G-1 cases (G-1a, G-1b,
  G-1c) will be observed if $h \in \ACA \cap \WCF$.
  \\
  G-1a (Aborted Reads) cannot be observed in $h$ because $h \in \ACA$ ensures that
  every read operation in history $h$ reads a committed value.
  \\
  G-1b (Intermediate Reads) cannot be observed since it is considered
  that a transaction can modify an object only once.
  \\
  By contradiction assume that $h \in \ACA \cap \WCF$ and G-1c
  (Circular Information Flow) is observed. Thus, there should be a directed
  cycle in DSG(h) containing only ww and wr dependency edges.\\
  Case a) There is a ww edge in the cycle between $T_i$ and $T_j$ while there is
  not a wr edge between them. Thus, $T_i \cc T_j \wedge ws(T_i) \cap
  ws(T_j) \neq \varnothing \Rightarrow h \notin \WCF$. A contradiction to the
  assumption. \\
  Case b) All the edges in the cycle are labeled with wr-dependency. It is
  straightforward to show that this phenomena violates the assumption that $h
  \in \ACA$. 
\end{IEEEproof}

\begin{proposition}
  \labprop{phenomena:3}
  If history $h$ belongs to $\ACA \inter \WCF$, then phenomenon G-SIa does not occur.
\end{proposition}

\begin{IEEEproof}
  An augmented history $S(h)$ exhibits phenomenon G-SIa
  if $SSG(S(h))$ contains a
  rw-dependency or ww-dependency edge from $T_i$ to $T_j$
  without there also being a start-dependency edge from $T_i$ to $T_j$ \cite{Adya2000}.
  
  Consider some history $h$ such that $h$ belongs to $\ACA \inter \WCF$.
  We prove that there exists a mapping $S$ such that $S(h)$ does not exhibit G-SIa.
  TBD.
%   by using \depend instead of \precedes.
%   Since \ACA implies that \depend is
%   acyclic, the above construction terminates.
%   Case a) assume by contradiction that there is only ww-dependency edge between
%   $T_i$ and $T_j$ without start or wr dependency edge from $T_j$ to
%   $T_i$. Thus, $T_i \cc T_j \wedge ws(T_i) \cap ws(T_j) \neq \varnothing
%   \Rightarrow h \notin \WCF$. A contradiction to the assumption that $h \in
%   \WCF$.
%   Case b) assume by contradiction that there is only wr-dependency edge between
%   $T_i$ and $T_j$ without start dependency edge from $T_j$ to
%   $T_i$. Therefore, the snapshot point of $T_i$ precedes the commit point of
%   $T_j$. Therefore, $r_i(x_j) <_{h} c_j$. A contradiction to the assumption that
%   $h \in \ACA$.   
\end{IEEEproof}
