# Supplementary material for: Non-Monotonic Snapshot Isolation
Source: arXiv:1306.3906 source file (2013-06-17)
Supplement: Supplementary file 3 [file proof_impossibility.tex]

\subsection{Proofs of Theorems \ref{theo:imp:1}, \ref{theo:imp:2} and \ref{theo:imp:3}}
\labappendix{impossibility}

In what follows, we consider some asynchronous failure-free \GPR system \procSet
satisfying the progress and safety requirements we described in \refsection{model}.
In \reflem{imp:1}, we characterize histories admissible by \procSet.
Then we prove our three impossibility results.
 
\begin{lemma}
  \lablem{imp:1}
  Let $h=\refMapOf{\run}$ be an admissible history such that a transaction $T_i$ is pending in $h$.
  Note $X$ the objects accessed by $T_i$ in $h$.
  Only processes in \replicaSetOf{X} make steps to execute $T_i$ in $\run$.
\end{lemma}

\begin{IEEEproof}
  By contradiction, assume that a process $p \notin \replicaSetOf{X}$ makes steps to execute $T_i$ in $\run$.
  Since the prefix of a transaction is a transaction with the same id, 
  we can consider an extension $\run'$ of $\run$ such that
  $T_i$ does not execute additional operations in $\run'$ and $\proxyOf{T_i}$ is correct in $\run'$.
  The progress requirements satisfied by \procSet imply that $T_i$ terminates in $\run'$ as well.
  However, process $p \notin \replicaSetOf{X}$  makes steps to execute $T_i$ in $\run'$.
  A contradiction to the fact that \procSet is GPR.
\end{IEEEproof}

\newtheorem*{theomon}{\reftheo{imp:1}}
\begin{theomon}
  No asynchronous failure-free \GPR system implements \MON.
\end{theomon}

\begin{IEEEproof}
  By contradiction. Let us consider,
  \begin{compactitem}
  \item Four objects $x$,$y$,$z$ and $u$ such that for any two objects in $\{x,y,z,u\}$,
    their replica sets do not intersect;
  \item Four queries $T_a$, $T_b$, $T_c$ and $T_d$
    accessing respectively $\{x,y\}$, $\{y,z \}$, $\{z,u\}$ and $\{u,x\}$; and
  \item Four update transactions $T_1$, $T_2$, $T_3$ and $T_4$
    modifying respectively $x$, $y$, $z$ and $u$.
  \end{compactitem}

  History $r_b(y_0)$ is admissible because \procSet implements non-trivial \SI.
  Since updates are obstruction-free, history $r_b(y_0).r_2(y_0).w_2(y_2).c_2$ is also admissible.
  Applying again that \procSet satisfies non-trivial \SI,
  we obtain that $r_b(y_0).r_2(y_0).w_2(y_2).c_2.r_a(y_2).r_a(x_0)$ is admissible.
  Since transaction $T_a$ is wait-free, history  $h=r_b(y_0).r_2(y_0).w_2(y_2).c_2.r_a(x_0).r_a(y_2).c_a$ is admissible as well.
  Using a symmetrical reasoning, we conclude that  $h'=r_d(u_0).r_4(u_0).w_4(u_4).c_4.r_c(z_0).r_c(u_4).c_c$ is also admissible.
  Let $\run$ and $\run'$ denote two sequences of steps 
  such that $\refMapOf{\run}=h$ and $\refMapOf{\run'}=h'$.

  Because updates are obstruction-free, history $h_1=h.h'.r_3(z_0).w_3(z_3).c_3$ is admissible.
  Since
  \emph{(i)} $T_b$ is pending in $h_1$,
  \emph{(ii)} concurrent transactions to $T_b$ in $h_1$, namely $T_a$ and $T_d$, 
      do not write-accesses $z$ or $y$,
  and
  \emph{(iii)} \procSet satisfies non-trivial \SI, 
  there exists a sequence of steps $U_1$ such that
  \emph{(i)} $\run.\run'.U_1$ extends $\run.\run'$,
  \emph{(ii)} $\refMapOf{U_1}$ equals $r_b(z_3).c_b$
  and \emph{(iii)} history $h_1.r_b(z_3).c_b$ is admissible.

  Applying a reasoning symmetrical to the one above,
  we note $U_2$ a sequence of steps such that
  \emph{(i)} $\run'.\run.U_2$ extends $\run'.\run$,
  \emph{(ii)} $\refMapOf{U_2}$ equals $r_d(x_1).c_d$,
  and \emph{(iii)} history $h'.h.r_1(x_0).w_1(x_1).c_1.r_d(x_1).c_d$ is admissible.

  Because \procSet satisfies \GPR, \reflem{imp:1} implies that only processes in
  $\replicaSetOf{x} \union \replicaSetOf{y}$ make steps in $\run$.
  Similarly, only processes in $\replicaSetOf{u} \union \replicaSetOf{z}$ make steps in $\run'$.
  By hypothesis, the set $\replicaSetOf{x} \union \replicaSetOf{y}$ and $\replicaSetOf{u} \union \replicaSetOf{z}$ are disjoint.
  As a consequence, Lemma~1 in \cite{Fischer1985} tells us that $\run.\run'$ and $\run.\run'$ are undistinguishable.
  Since $\run'.\run.U_2$ is admissible, 
  it follows that $\run.\run'.U_2$ is also admissible.

  Executions $\run.\run'.U_1$ and $\run.\run'.U_2$ are both admissible.
  Because \procSet is \GPR,
  only processes in $\replicaSetOf{y} \union \replicaSetOf{z}$ execute steps in $U_1$.
  Similarly in $U_2$, only processes in $\replicaSetOf{x} \union \replicaSetOf{u}$ make steps.
  By hypothesis, these two replica sets are disjoint.
  It follows that execution $\run.\run'.U_1.U_2$ is undistinguishable from $\run.\run'.U_1$ (resp. $\run.\run'.U_2$)
  for the processes in $\replicaSetOf{y} \union \replicaSetOf{z}$ (resp. $\replicaSetOf{x} \union \replicaSetOf{u}$).
  As a consequence, $\run.\run'.U_1.U_2$ is an execution of \procSet.
  Therefore, $\hat{h}=h'.h.r_1(x_0).w_1(x_1).c_1.r_d(x_1).c_d.r_3(z_0).w_3(z_3).c_3.r_b(z_3).c_b$ is admissible.

  According to the precedence relation between snapshots,
  we observe that in history $\hat{h}$ we have the relation:
  $T_a \rightarrow T_b \rightarrow T_c \rightarrow T_d \rightarrow T_a$.
  Hence, this execution violates \MON.
  Contradiction. 
\end{IEEEproof}

We now turn our attention to the cost of computing strictly consistent snapshots.
We first state that a choice must be made between \SCONSb and \GPR.
This result follows a schema similar to the proof of Theorem~4 in \cite{Attiya:SPAA2009}:
We construct an infinite execution of a read-only transaction $T_a$ that never terminates.
During the execution, we interleave between any two consecutive steps to execute $T_a$, 
a transaction updating one of the objects read by $T_a$.
We first define a special (finite) execution of this form, called flippable \citep{Attiya:SPAA2009},
and show that during such an execution, transaction $T_a$ does not terminate successfully (\reflem{imp:2}).
Then, we prove that if no synchrony assumptions holds, we can extend the flippable execution \emph{ad eternam},
contradicting the fact that read-only transactions are wait-free.

\begin{definition*}[Flippable execution]
  Consider
  two distinct objects $x$ and $y$,
  a read-only transaction $T_a$ over both objects,
  and a set of updates $T_{j \in \llbracket 1,m \rrbracket}$ accessing $x$ if $j$ is odd, and $y$ otherwise.
  An execution $\run=U_1s_2U_2s_2 \ldots s_mU_m$ where,
  \begin{itemize}
    \item transaction $T_a$ reads in history $h=\mathfrak{F}(\run)$ at least (in the sense of $\versionOrder_h$) version $x_1$ of $x$,
    \item $s_{j \in \llbracket 1,m \rrbracket}$ is a single step to execute $T_a$ by some process $p_j$,
    \item $U_{j \in \llbracket 1,m \rrbracket}$ is the execution of transaction $T_j$ by some set of processes $Q_j$, and 
    \item for any $j$ in $\llbracket 1,m \llbracket$, $Q_j \inter Q_{j+1} = \emptySet$ holds,
  \end{itemize}
  is called \emph{flippable}.
\end{definition*}

\begin{lemma}
  \lablem{imp:2}
  In a flippable execution $\run$ satisfying $\mathfrak{F}(\run) \in \SCONSb$,
  query $T_a$ does not terminate 
\end{lemma}

\begin{IEEEproof}
  Let $h$ be the history $\mathfrak{F}(\run)$.
  In history $h$ transaction $T_j$ precedes transaction $T_{j+1}$,
  it follows that $h$ is of the form $h=w_1(x_1).c_1. *. w_2(y_2).c_2.* \ldots$\ ,
  where each symbol $*$ correspond to either no operation, or to some read operation 
  by $T_a$ on either object $x$, or $y$.

  Because \run is flippable, transaction $T_a$ reads at least version $x_1$ of object $x$ in $h$.
  For some odd natural  $j \geq 1$,  let $x_j$ denote the version of object $x$ read by $T_a$.
  Similarly, for some even natural $l$, let $y_{l}$ be the version of $y$ read by $T_a$.
  Assume that $k<l$ holds.
  Therefore, $h$ is of the form $h=\ldots  w_{j}(x_{j}) \ldots w_l(y_l) \ldots$.

  Note $k$ the value $l+1$, 
  and consider the step $s_k$ made by $p_k$ right after $U_{l}$ to execute $T_a$.
  According to the definition of a flippable execution, we know that:
  (F1) $p_k \in Q_l \xor p_k \in Q_k$,
  and (F2) $Q_l \inter Q_k \equals \emptySet$.
  Consider the following cases:
  \begin{compactitem}
  \item[(\textsc{Case $p_k \in Q_k$.})] ~
    Applying fact F1, execution $\run$ is indistinguishable from $\run''=\ldots
    U_j \ldots s_{k} U_l U_k \ldots$. Then applying fact F2, $\run$ is
    indistinguishable from execution $\run'=\ldots U_j \ldots s_{k} U_k U_l \ldots$.
  \item[(\textsc{Case $p_k \in Q_l$.})]~
    With a similar reasoning, we obtain that $\run$ is indistinguishable from
    $\run'=\ldots U_j \ldots U_k U_l s_k \ldots$.
  \item[(\textsc{Case $p_k \notin Q_l \union Q_k$.})]~
    This case reduces to any of the two above cases.
  \end{compactitem}
  Note $h'$ the history $\mathfrak{F}(\run')$.
  In history $\run'$, 
  both $w_k(x_k) <_{h'} w_l(y_l)$ and $x_j \versionOrder_{h'} x_k$ hold.
  Besides, operations  $r_i(x_j)$, $r_i(y_l)$ and $w_k(x_k)$ all belong to $h'$.
  Thus, history $h'$ does not belong to \SCONSb, or transaction $T_a$ does not commit in $h'$.
  Since $\run'$ is indistinguishable from $\run$, history $h'$ is admissible.
  It follows that $T_a$ does not commit in $h'$.
  (The case $k>l$ follows a symmetrical reasoning to the case $l>k$ we considered previously.)
\end{IEEEproof}

\newtheorem*{theosconsb}{\reftheo{imp:2}}
\begin{theosconsb}
  No asynchronous failure-free \GPR system implements \SCONSb.
\end{theosconsb}

\begin{IEEEproof}
  Consider some read-only transaction $T_a$, 
  two distinct objects $x$ and $y$ read by $T_a$,
  and assume that $\replicaSetOf{x}$ and $\replicaSetOf{y}$  are disjoint.

  We reason by contradiction,
  exhibiting an admissible execution during which transaction $T_a$ never terminates.
  This execution is constructed as follows:

  \paragraph{Construction.}
  Let $\mathcal{P}$ be an initially empty FIFO list, and consider an initially null execution $\run$.
  Start executing $T_a$ by \coordOf{T_a}.
  Repeat for all $i \geq 1$.
  Add to $\mathcal{P}$ (in some arbitrary order) 
  the processes that have to execute a step for $T_a$.
  Pop from $\mathcal{P}$ the next process $p$ to execute a step for $T_a$.
  Extend $\run$ with step $s_i$, the next step of $p$.
  Let $T_i$ be an update of $x$, if $i$ is even, and $y$ otherwise.
  Start the execution of transaction $T_i$.
  Since 
  no transaction are concurrent, 
  updates are obstruction-free
  and the system is genuine, 
  there exists an extension $\run' = \run \cseqAppend U_i$ during which $T_i$ commits
  and such that in $U_i$, 
  only processes in \replicaSetOf{x}, if $i$ is odd, or in \replicaSetOf{y} otherwise, execute steps.
  Assign to $\run$ the value of $\run'$.

  By construction, execution $\run$ is flippable.
  Hence, \reflem{imp:2} tells us that transaction $T_a$ does not terminate in this run.
  Since every process in $\mathcal{P}$ eventually make a step in $\run$, $\run$ is fair.
  Because there is no synchrony assumptions, this execution is admissible.
  In \run, transaction $T_a$ never commits.
  Contradiction.
\end{IEEEproof}

\bigskip
\noindent
Our last impossibility result circumvents the cost of \SCONSa.

\newtheorem*{theosconsa}{\reftheo{imp:3}}
\begin{theosconsa}
  No asynchronous failure-free \GPR system implements \SCONSa.
\end{theosconsa}

\begin{IEEEproof}
  Consider two distinct objects $x$ and $y$ such that $\replicaSetOf{x}$ and $\replicaSetOf{y}$ are disjoint.
  Let $T_1$ be an update transaction accessing $x$, 
  $T_2$ be an update on $y$,
  and $T_a$ be a read-only transaction accessing both objects.
  
  Since updates are obstruction-free, history $h_1=r_1(x_0).w_1(x_1).c_1$ is admissible.
  Let $U_1$ be a sequence of steps such that $\refMapOf{U_1}=r_1(x_0).w_1(x_1).c_1$.

  The system \procSet satisfies non-trivial \SI.
  Consequently, there exists an extension $U_1.U_a$ of $U_1$ such that $\refMapOf{U_a}=r_a(x_1)$, 
  and history $h_2=h_1.\refMapOf{U_a}$ is admissible.

  Then, since the system supports obstruction-free updates,
  there exists an extension $U_1.U_a.U_2$ such that 
  $\refMapOf{U_2}=r_2(y_0).w_2(y_2)$, and history $h_3=h_2.\refMapOf{U_2}$ is admissible.

  Finally, we may extend $U_1.U_a.U_2$ by a sequence of steps $V_a$ such that 
  $\refMapOf{V_a}=r_a(y_2).c_2$, and $h_3.\refMapOf{V_a}$ is admissible.
  Such an extension is possible 
  since \procSet satisfies both non-trivial SI and wait-free queries.
  
  Consider the execution $U_1.U_a.U_2$.
  Applying \reflem{imp:1}, 
  only processes in \replicaSetOf{x} make steps to execute $T_a$ in this execution.
  Since \replicaSetOf{x} and \replicaSetOf{y} are disjoint, 
  it follows that $U_1.U_a.U_2$ is indistinguishable from $U_1.U_2.U_a$.
  As a consequence, the execution $U_1.U_2.U_a.V_a$ is admissible.
  Notice that $\refMapOf{U_1.U_2.U_a.V_a}$ equals 
  $r_1(x_0).w_1(x_1).c_1.r_a(x_1).r_2(y_0).w_2(y_2).r_a(y_2).c_2$.
  This history is not in \SCONSa.
  Contradiction.
\end{IEEEproof}
