# Supplementary material for: Non-Monotonic Snapshot Isolation
Source: arXiv:1306.3906 source file (2013-06-17)
Supplement: Supplementary file 4 [file appendix.tex]

\subsection{Proof of \reftheo{reconstruct:main}}
\labappendix{reconstruct}

In \reftheo{reconstruct:main}, we claim that $\SI$ equals
the intersection of $\ACA$, $\SCONS$, $\WCF$ and $\MON$.
This section is devoted to a rigorous proof of this claim.
\refprop{reconstruct:1} states that  $\SI \subseteq \ACA \inter \SCONS \inter \WCF \inter \MON$ holds.
In \refprop{reconstruct:2}, we prove that the converse is true.
We start our proof by the three technical lemmata bellow.

\begin{lemma}
  \lablem{reconstruct:1}
  Consider a history $h \in \SI$ and two versions $x_i$ and $x_j$ of some object $x$.
  If $x_i \versionOrder_{h} x_j$ holds then $T_j \depend T_i$ is true.
\end{lemma}

\begin{proof}
  Assume some history $h \in \SI$ such that $x_i \versionOrder_h x_j$ holds.
  Let $h_s$ be an extended history for $h$ that satisfies rules D1 and D2.
  According to the model, transaction $T_j$ first reads some version $x_k$, then writes version $x_j$.

  First, assume that there is no write to $x$ between $w_i(x_i)$ and $w_j(x_j)$.
  Since $x$ belongs to $\writeSetOf{T_i} \inter \writeSetOf{T_j}$,
  rule D2 tells us that either $c_i <_{h_s} s_j$, or  $c_j <_{h_s} s_i$ holds.
  We observe that because $x_i \versionOrder_h x_j$ holds, it must be true that $c_i <_{h_s} s_j$.
  Since there is no write to $x$ between $w_i(x_i)$ and $w_j(x_j)$, $x_k \versionOrder x_i$ holds, or $k=i$.
  Observe that in the former case rule D1.3 is violated.
  Thus, transaction $T_j$ reads version $x_i$.
  
  To obtain the general case, we apply inductively the previous reasoning.
\end{proof}
 
\begin{lemma}
  \lablem{reconstruct:2}
  Let $h \in \SI$ be an history, 
  and $\mathcal{S}$ be a function such that $h_s=\mathcal{S}(h)$ satisfies D1 and D2.
  Consider $T_i, T_j \in h$.
  If $T_i \rightarrow T_j$ holds then $s_i <_{h_s} s_j$.
\end{lemma}

\begin{proof}
  Consider two transactions $T_i$ and $T_j$ such that the snapshot of $T_i$ precedes the snapshot of  $T_j$.
  By definition of the snapshot precedence relation, 
  there exist $T_k, T_l \in h$ such that $r_i(x_k), r_j(y_l) \in h$ and
  either \emph{(i)} $r_i(x_k) <_h c_l$\ , 
  or \emph{(ii)} $w_l(x_l) \in h$ and $c_k <_h c_l$.
  Let us distinguish each case:
  \begin{compactitem}
  \item[(Case $r_i(x_k) <_h c_l$)]
    By definition of function $\mathcal{S}$, $s_i$ precedes $r_i(x_k)$ in $h_s$.
    From $r_j(y_l) \in h$ and rule D1.2, $c_l <_{h_s} s_j$ holds.
    Hence, $s_i <_{h_s} s_j$ holds.
  \item[(Case $c_k <_h c_l$)]
    From \emph{(i)} $r_i(x_k), w_l(x_l) \in h$, \emph{(ii)} $c_k <_h c_l$ and \emph{(iii)} rule D1.3, 
    we obtain $s_i <_{h_s} c_l$.
    From $r_j(y_l) \in h$ and rule D1.2, $c_l <_{h_s} s_j$ holds.
    It follows that $s_i <_{h_s} s_j$ holds.
  \end{compactitem}
\end{proof}

\begin{lemma}
  \lablem{reconstruct:3}
  Consider a history $h \in \ACA \inter \CONS \inter \WCF$, and two versions $x_i$ and $x_j$ of some object $x$. 
  If $x_i \versionOrder_h x_j$ holds then $c_i <_h c_j$.
\end{lemma}

\begin{proof}
  Since both $T_i$ and $T_j$ write to $x$ and $h$ belongs to $\WCF$
  either $T_j \depend T_i$ or $T_i \depend T_j$ holds.
  We distinguish the two cases below:
  \begin{compactitem}
  \item[(Case $T_j \depend T_i$)]
    First, assume that $T_j \MustHave T_i$ holds.
    Note $y$ an object such that $r_j(y_i)$ is in $h$.
    Since $h$ belongs to $\ACA$, $c_i <_h r_j(y_i)$ holds.
    Because $h$ is an history, $r_j(y_i) <_h c_j$ must hold.
    Hence we obtain $c_i <_h c_j$.
    By a short induction, we obtain the general case. 
  \item[(Case $T_i \depend T_j$)]
    Let us note $x_k$ the version of $x$ read by transaction $T_i$.
    From the definition of an history and since $h$ belongs to to \ACA, we know that
    $w_k(x_k) <_h c_k <_h r_i(x_k) <_h w_i(x_i)$ holds.
    As a consequence, $x_k \versionOrder_h x_i$ is true.
    Since
    \emph{(i)} $h$ belongs to \CONS, 
    \emph{(ii)} $T_i \depend T_j$,
    and \emph{(iii)} $T_j$ writes to $x$,
    it must be the case that $x_j \versionOrder_h x_k$.
    We deduce that $x_j \versionOrder_h x_i$ holds; a contradiction.
  \end{compactitem}
\end{proof}

\begin{proposition}
  \labprop{reconstruct:1}
  $\SI \subseteq \ACA \inter \SCONS \inter \WCF \inter \MON$
\end{proposition}

\begin{proof}
  Choose $h$ in \SI.
  Note $\mathcal{S}$ a function such that history $h_s=\mathcal{S}(h)$ satisfies rules D1 and D2.

  \begin{compactitem}

  \item[($h \in \ACA$)]
    It is immediate from rules D1.1 and D1.2. 

  \item[($h \in \WCF$)]
    Consider two independent transactions $T_i$ and $T_j$ modifying the same object $x$.
    By the definition of an history, $x_i \versionOrder_h x_j$ \ , or $x_j \versionOrder_h x_i$ holds.
    Applying \reflem{reconstruct:1}, we conclude that in the former case $T_j$ depends on $T_i$,
    and that the converse holds in the later.

  \item[($h \in \SCONSa$)]
    By contradiction.
    Assume three transactions $T_i$, $T_j$ and $T_l$ such that
    $r_i(x_j), r_i(y_l) \in h$ and $r_i(x_j) <_h c_l$ are true.
    In $h_s$, the snapshot point $s_i$ of transaction $T_i$ is placed prior to every operation of $T_i$ in $h_s$.
    Hence, $s_i$ precedes $r_i(x_j)$ in $h_s$.
    This implies that  $s_i <_{h_s} c_l \land r_i(y_l) \in h_s$ holds.
    A contradiction to rule D1.2.
    
  \item[($h \in \SCONSb$)]
    Assume for the sake of contradiction four transactions $T_i$, $T_j$, $T_{k \neq j}$ and $T_l$
    such that: $r_i(x_j), r_i(y_l)$,  $w_k(x_k) \in h$, $c_k <_h c_l$ and $c_k \not<_{h} c_j$ are all true.
    Since transaction $T_j$ and $T_k$ both write $x$, by rule D2, we know that $c_j <_{h_s} c_k$ holds.
    Thus, $c_j <_{h_s} c_k <_{h_s} c_l$ holds.
    According to rule D1.2, since $r_i(y_l)$ is in $h$, $c_l <_{h_s} s_i$ is true.
    We consequently obtain that $c_j <_{h_s} c_k < s_i$ holds.
    A contradiction to rule D1.3.

  \item[($h \in MON$)]
    If \precedes is not a  partial order, there exist transactions $T_1, \ldots, T_{n \geq 1}$ 
    such that: $T_1 \rightarrow \ldots \rightarrow T_n \rightarrow T_1$.
    Applying \reflem{reconstruct:2}, we obtain that the relation $s_1 <_{h_s} s_1$ is true.
    A contradiction.

  \end{compactitem}
\end{proof}

\begin{proposition}
  \labprop{reconstruct:2}
  $\ACA \inter \SCONS \inter \WCF \inter \MON \subseteq \SI$
\end{proposition}

\begin{proof}
  Consider some history $h$ in $\ACA \inter \SCONS \inter \WCF \inter \MON$.
  If history $h$ belongs to $\SI$ 
  then there must exist a function $\mathcal{S}$ such that  $h'=\mathcal{S}(h)$ satisfies rules D1 and D2. 
  In what follows, we build such an extended history $h'$, then we prove its correctness.

  \vspace{0.5em}
  \noindent
  [Construction]
  Initially $h'$ equals $h$.
  For every transaction $T_i$ in $h'$ we add a snapshot point $s_i$ in $h'$,
  and for every operation $o_i$ in $h'$, we execute the following steps:
  \begin{compactitem}
  \item[\textbf{S1.}] We add the order $(s_i,o_i)$ to $h'$.
  \item[\textbf{S2.}] If $o_i$ equals $r_i(x_j)$ for some object $x$ then
    \begin{compactitem}
    \item[\textbf{S2a.}] we add the order $(c_j,s_i)$ to $h'$,
    \item[\textbf{S2b.}] and, for every committed transaction $T_k$ such that $w_k(x_k)$ is in $h$,
          if $c_k <_{h} c_j$ does not hold then we add the order $(s_i,c_k)$ to $h'$.
    \end{compactitem}
  \end{compactitem}
  
  \vspace{0.5em}
  \noindent
  [Correctness]
  We now prove that $h'$ is an extended history that satisfies rules D1 and D2.
  \begin{itemize}

  \item $h'$ is an extended history.

    Observe that for every transaction $T_i$ in $h'$, there exists a snapshot point $s_i$,
    and that according to step S1, $s_i$ is before all operations of transaction $T_i$.
    It remains to show that order $<_{h'}$ is acyclic.
    We proceed by contradiction.

    Since $h$ is a history, it follows that any cycle formed by relation $<_{h'}$  contains a snapshot point $s_i$.
    Furthermore, according to steps S1 and S2 above, we know that for some operation $c_{j \neq i}$,
    relation $c_j <_{h'} s_i <_{h'}^* c_j$ holds.

    By developing relation $s_i <_{h'}^* c_j$, we obtain the following three relations.
    The first two relations are terminal, while the last is recursive.
    \begin{compactitem}
    \item Relation $s_i <_{h'} c_j$ holds.
      This relation has to be produced by step S2b.
      Hence, there exist operations $r_i(x_k), w_j(x_j)$ in $h'$ such that $c_j <_h c_k$ does not hold.
      Observe that since $h$ belongs to $\ACA \inter \CONS \inter \WCF$, 
      by \reflem{reconstruct:3}, it must be the case that  $c_k <_h c_j$ holds.
    \item Relation $s_i <_{h'} o_i <_h^* c_j$ holds for some read operation $o_i$ in $T_i$.
      (If $o_i <_h^* c_j$ with $o_i$ a write or a terminating operation, 
      we may consider a preceding read that satisfies the same relation.)
    \item Relation $s_i <_{h'} o_i <_{h'}^* c_j$ holds for some read operation $o_i$ in $T_i$,
      and $o_i <_{h'}^* c_j$ does not imply  $o_i <_h^* c_j$.
      (Again if $o_i$ is a write or a terminating operation, we may consider a preceding read that satisfies this relation.)
      Relation $o_i <_{h'}^* c_j$ cannot be produced by steps S1 and S2.
      Hence, there must exist a commit operation $c_k$ and a snapshot point $s_l$ such that
      $s_i <_{h'} o_i <_h c_k <_{h'} s_l <_{h'}^* c_j$ holds.
    \end{compactitem}
    From the result above, we deduce that there exist
    snapshot points $s_1, \ldots, s_{n \geq 1}$ and commit points $c_{k_1} \ldots c_{k_n}$ such that:
    \begin{equation}
      \labequation{reconstruct:1}
      s_1 \hb c_{k_1} <_{h'} s_2 \hb c_{k_2} \ldots s_n \hb c_{k_n} <_{h'} s_1
    \end{equation}
    where $s_i \hb c_{k_i}$ is a shorthand for 
    either \emph{(i)} $s_i <_{h'} c_{k_i}$ with $r_i(x_j), w_{k_i}(x_{k_i}) \in h$ and $c_j <_h c_{k_i}$,
    or \emph{(ii)} $s_i <_{h'} o_i <_h c_{k_i}$ with $o_i$ is some read operation.

    We now prove that for every $i$,  $T_i \rightarrow T_{i+1}$ holds.
    Consider some $i$.
    First of all, observe that a relation $c_{k_{i-1}} < s_i$ is always produced by step S2a.
    Then, since relation $s_i \hb c_{k_i} <_{h'} s_{i+1}$ holds we may consider the two following cases:
    \begin{compactitem}
    \item Relation $s_i <_{h'} c_{k_i} <_{h'} s_{i+1}$ holds  with $r_i(x_j), w_{k_i}(x_{k_i}) \in h$ and $c_j <_h c_{k_i}$.
      From $c_{k_i} <_{h'} s_{i+1}$ and step S2a, there exists an object $y$ such that $r_{i+1}(y_{k_i})$.
      Thus, by definition of the snapshot precedence relation, $T_i \rightarrow T_{i+1}$ holds.
    \item Relation $s_i \hb c_{k_i}$ equals $s_i <_{h'} o_i <_h c_{k_i}$ where $o_i$ is some read operation of $T_i$,
      Since $c_{k_i} <_{h'} s_{i+1}$ is produced by step S2a, we know that for some object $y$, 
      $r_{i+1}(y_{k_i})$ belongs to $h$.
      According to the definition of the snapshot precedence, $T_i \rightarrow T_{i+1}$ holds.
    \end{compactitem}

    Applying the result above to \refequation{reconstruct:1}, we obtain:
    $T_1 \rightarrow T_2 \ldots \rightarrow T_n \rightarrow T_1$.
    History $h$ violates \MON, a contradiction.

  \item  $h'$ satisfies rules D1 and D2.
    
    \begin{compactitem}[$-$]
      
    \item[($h'$ satisfies D1.1)]
      Follows from $h \in \ACA$,

    \item[($h'$ satisfies D1.2)]
      Immediate from step S1.

    \item[($h'$ satisfies D1.3)]
      Consider three transactions $T_i$, $T_j$ and $T_k$ such that 
      operations $r_i(x_j)$, $w_j(x_j)$ and $w_k(x_k)$ are in $h$.
      The definition of an history tells us that either $x_k \versionOrder_h x_j$
      or the converse holds.
      We consider the following two cases:
      \begin{compactitem}
      \item[(Case $x_k \versionOrder_h x_j$)]
        Since $h$ belongs to $\ACA \inter \CONS \inter \WCF$, 
        \reflem{reconstruct:3} tells us that $c_k <_h c_j$ holds.
        Hence, $c_k <_{h'} c_j$ holds.
      \item[(Case  $x_j \versionOrder_h x_k$)]
        Applying again \reflem{reconstruct:3}, we obtain that  $c_j <_h c_k$ holds.
        Since $<_h$ is a partial order, then $c_j <_{h} c_k$ does not hold.
        By step S2b, the order $(s_i,c_k)$ is in $h'$.
      \end{compactitem}
      
    \item[($h'$ satisfies D2)]
      Consider two conflicting transaction $(T_i,T_j)$ in $h'$.
      Since $h$ belongs to  $\WCF$, 
      one of the following two cases occurs:
      \begin{compactitem}
      \item[(Case $T_i \depend T_j$)]
        At first glance, assume that $T_i \depend T_j$ holds.
        By step S2a, $s_i$ is in $h'$ after every operation $c_j$ such that $r_i(x_j)$ is in $h'$,
        and by step S1, $s_i$ precedes the first operation of $T_i$.
        Thus $c_j <_{h'} s_i$ holds, and $h'$ satisfies D2 in this case. 
        To obtain the general case, we applying inductively the previous reasoning.
      \item[(Case $T_j \depend T_i$)]
        The proof is symmetrical to the case above, and thus omitted.
      \end{compactitem}

    \end{compactitem}

  \end{itemize}

\end{proof}

\noindent
From the conjunction of \refprop{reconstruct:1} and \refprop{reconstruct:2}, we deduce that:

\newtheorem*{theoreconstruct}{\reftheo{reconstruct:main}}
\begin{theoreconstruct}
  $\SI = \SCONS \inter \MON \inter \WCF \inter \ACA$
\end{theoreconstruct}

\noindent
This decomposition is \emph{well-formed} in the sense that 
the four properties \SCONS, \MON, \WCF and \ACA are distinct
and that no strict subset of $\{\SCONS, \MON, \WCF, \ACA \}$ attains \SI.

\begin{proposition}
  For every $S \subsetneq \{\SCONS, \MON, \WCF, \ACA \}$, 
  it is true that $\inter_{X \in S} X \neq \SI$.
\end{proposition}

\begin{proof}  
  For every set $S \subsetneq \{\SCONS, \MON, \WCF, \ACA \}$ containing three of the four properties, 
  we exhibit below an history in $\inter_{X \in S} X \setminus \SI$.
  Trivially, the result then holds for every $S$.
  ($\SCONS \inter \ACA \inter \WCF$) History $h_6$ in \refsection{reconstruct}.
  ($\MON \inter \ACA \inter \WCF$) History $h_5$ in \refsection{reconstruct}
  ($\SCONS \inter \MON \inter \WCF$) History $r_1(x_0).w_1(x_1).r_a(x_0).c_1.c_a$.
  ($\SCONS \inter \MON \inter \ACA$) History $r_1(x_0).r_2(x_0).w_1(x_1).w_2(x_2).c_1.c_2$
\end{proof}

\newpage
\subsection{Proofs of Theorems \ref{theo:imp:1}, \ref{theo:imp:2} and \ref{theo:imp:3}}
\labappendix{impossibility}

In what follows, we consider some asynchronous failure-free \GPR system \procSet
satisfying the progress and safety requirements we described in \refsection{model}.
In \reflem{imp:1}, we characterize histories admissible by \procSet.
Then we prove our three impossibility results.
 
\begin{lemma}
  \lablem{imp:1}
  Let $h=\refMapOf{\run}$ be an admissible history such that a transaction $T_i$ is pending in $h$.
  Note $X$ the objects accessed by $T_i$ in $h$.
  Only processes in \replicaSetOf{X} make steps to execute $T_i$ in $\run$.
\end{lemma}

\begin{IEEEproof}
  By contradiction, assume that a process $p \notin \replicaSetOf{X}$ makes steps to execute $T_i$ in $\run$.
  Since the prefix of a transaction is a transaction with the same id, 
  we can consider an extension $\run'$ of $\run$ such that
  $T_i$ does not execute additional operations in $\run'$ and $\proxyOf{T_i}$ is correct in $\run'$.
  The progress requirements satisfied by \procSet imply that $T_i$ terminates in $\run'$ as well.
  However, process $p \notin \replicaSetOf{X}$  makes steps to execute $T_i$ in $\run'$.
  A contradiction to the fact that \procSet is GPR.
\end{IEEEproof}

\newtheorem*{theomon}{\reftheo{imp:1}}
\begin{theomon}
  No asynchronous failure-free \GPR system implements \MON.
\end{theomon}

\begin{IEEEproof}
  By contradiction. Let us consider,
  \begin{compactitem}
  \item Four objects $x$,$y$,$z$ and $u$ such that for any two objects in $\{x,y,z,u\}$,
    their replica sets do not intersect;
  \item Four queries $T_a$, $T_b$, $T_c$ and $T_d$
    accessing respectively $\{x,y\}$, $\{y,z \}$, $\{z,u\}$ and $\{u,x\}$; and
  \item Four update transactions $T_1$, $T_2$, $T_3$ and $T_4$
    modifying respectively $x$, $y$, $z$ and $u$.
  \end{compactitem}

  History $r_b(y_0)$ is admissible because \procSet implements non-trivial \SI.
  Since updates are obstruction-free, history $r_b(y_0).r_2(y_0).w_2(y_2).c_2$ is also admissible.
  Applying again that \procSet satisfies non-trivial \SI,
  we obtain that $r_b(y_0).r_2(y_0).w_2(y_2).c_2.r_a(y_2).r_a(x_0)$ is admissible.
  Since transaction $T_a$ is wait-free, history  $h=r_b(y_0).r_2(y_0).w_2(y_2).c_2.r_a(x_0).r_a(y_2).c_a$ is admissible as well.
  Using a symmetrical reasoning, we conclude that  $h'=r_d(u_0).r_4(u_0).w_4(u_4).c_4.r_c(z_0).r_c(u_4).c_c$ is also admissible.
  Let $\run$ and $\run'$ denote two sequences of steps 
  such that $\refMapOf{\run}=h$ and $\refMapOf{\run'}=h'$.

  Because updates are obstruction-free, history $h_1=h.h'.r_3(z_0).w_3(z_3).c_3$ is admissible.
  Since
  \emph{(i)} $T_b$ is pending in $h_1$,
  \emph{(ii)} concurrent transactions to $T_b$ in $h_1$, namely $T_a$ and $T_d$, 
      do not write-accesses $z$ or $y$,
  and
  \emph{(iii)} \procSet satisfies non-trivial \SI, 
  there exists a sequence of steps $U_1$ such that
  \emph{(i)} $\run.\run'.U_1$ extends $\run.\run'$,
  \emph{(ii)} $\refMapOf{U_1}$ equals $r_b(z_3).c_b$
  and \emph{(iii)} history $h_1.r_b(z_3).c_b$ is admissible.

  Applying a reasoning symmetrical to the one above,
  we note $U_2$ a sequence of steps such that
  \emph{(i)} $\run'.\run.U_2$ extends $\run'.\run$,
  \emph{(ii)} $\refMapOf{U_2}$ equals $r_d(x_1).c_d$,
  and \emph{(iii)} history $h'.h.r_1(x_0).w_1(x_1).c_1.r_d(x_1).c_d$ is admissible.

  Because \procSet satisfies \GPR, \reflem{imp:1} implies that only processes in
  $\replicaSetOf{x} \union \replicaSetOf{y}$ make steps in $\run$.
  Similarly, only processes in $\replicaSetOf{u} \union \replicaSetOf{z}$ make steps in $\run'$.
  By hypothesis, the set $\replicaSetOf{x} \union \replicaSetOf{y}$ and $\replicaSetOf{u} \union \replicaSetOf{z}$ are disjoint.
  As a consequence, Lemma~1 in \cite{Fischer1985} tells us that $\run.\run'$ and $\run.\run'$ are undistinguishable.
  Since $\run'.\run.U_2$ is admissible, 
  it follows that $\run.\run'.U_2$ is also admissible.

  Executions $\run.\run'.U_1$ and $\run.\run'.U_2$ are both admissible.
  Because \procSet is \GPR,
  only processes in $\replicaSetOf{y} \union \replicaSetOf{z}$ execute steps in $U_1$.
  Similarly in $U_2$, only processes in $\replicaSetOf{x} \union \replicaSetOf{u}$ make steps.
  By hypothesis, these two replica sets are disjoint.
  It follows that execution $\run.\run'.U_1.U_2$ is undistinguishable from $\run.\run'.U_1$ (resp. $\run.\run'.U_2$)
  for the processes in $\replicaSetOf{y} \union \replicaSetOf{z}$ (resp. $\replicaSetOf{x} \union \replicaSetOf{u}$).
  As a consequence, $\run.\run'.U_1.U_2$ is an execution of \procSet.
  Therefore, $\hat{h}=h'.h.r_1(x_0).w_1(x_1).c_1.r_d(x_1).c_d.r_3(z_0).w_3(z_3).c_3.r_b(z_3).c_b$ is admissible.

  According to the precedence relation between snapshots,
  we observe that in history $\hat{h}$ we have the relation:
  $T_a \rightarrow T_b \rightarrow T_c \rightarrow T_d \rightarrow T_a$.
  Hence, this execution violates \MON.
  Contradiction. 
\end{IEEEproof}

We now turn our attention to the cost of computing strictly consistent snapshots.
We first state that a choice must be made between \SCONSb and \GPR.
This result follows a schema similar to the proof of Theorem~4 in \cite{Attiya:SPAA2009}:
We construct an infinite execution of a read-only transaction $T_a$ that never terminates.
During the execution, we interleave between any two consecutive steps to execute $T_a$, 
a transaction updating one of the objects read by $T_a$.
We first define a special (finite) execution of this form, called flippable \citep{Attiya:SPAA2009},
and show that during such an execution, transaction $T_a$ does not terminate successfully (\reflem{imp:2}).
Then, we prove that if no synchrony assumptions holds, we can extend the flippable execution \emph{ad eternam},
contradicting the fact that read-only transactions are wait-free.

\begin{definition*}[Flippable execution]
  Consider
  two distinct objects $x$ and $y$,
  a read-only transaction $T_a$ over both objects,
  and a set of updates $T_{j \in \llbracket 1,m \rrbracket}$ accessing $x$ if $j$ is odd, and $y$ otherwise.
  An execution $\run=U_1s_2U_2s_2 \ldots s_mU_m$ where,
  \begin{itemize}
    \item transaction $T_a$ reads in history $h=\mathfrak{F}(\run)$ at least (in the sense of $\versionOrder_h$) version $x_1$ of $x$,
    \item $s_{j \in \llbracket 1,m \rrbracket}$ is a single step to execute $T_a$ by some process $p_j$,
    \item $U_{j \in \llbracket 1,m \rrbracket}$ is the execution of transaction $T_j$ by some set of processes $Q_j$, and 
    \item for any $j$ in $\llbracket 1,m \llbracket$, $Q_j \inter Q_{j+1} = \emptySet$ holds,
  \end{itemize}
  is called \emph{flippable}.
\end{definition*}

\begin{lemma}
  \lablem{imp:2}
  In a flippable execution $\run$ satisfying $\mathfrak{F}(\run) \in \SCONSb$,
  query $T_a$ does not terminate 
\end{lemma}

\begin{IEEEproof}
  Let $h$ be the history $\mathfrak{F}(\run)$.
  In history $h$ transaction $T_j$ precedes transaction $T_{j+1}$,
  it follows that $h$ is of the form $h=w_1(x_1).c_1. *. w_2(y_2).c_2.* \ldots$\ ,
  where each symbol $*$ correspond to either no operation, or to some read operation 
  by $T_a$ on either object $x$, or $y$.

  Because \run is flippable, transaction $T_a$ reads at least version $x_1$ of object $x$ in $h$.
  For some odd natural  $j \geq 1$,  let $x_j$ denote the version of object $x$ read by $T_a$.
  Similarly, for some even natural $l$, let $y_{l}$ be the version of $y$ read by $T_a$.
  Assume that $k<l$ holds.
  Therefore, $h$ is of the form $h=\ldots  w_{j}(x_{j}) \ldots w_l(y_l) \ldots$.

  Note $k$ the value $l+1$, 
  and consider the step $s_k$ made by $p_k$ right after $U_{l}$ to execute $T_a$.
  According to the definition of a flippable execution, we know that:
  (F1) $p_k \in Q_l \xor p_k \in Q_k$,
  and (F2) $Q_l \inter Q_k \equals \emptySet$.
  Consider the following cases:
  \begin{compactitem}
  \item[(\textsc{Case $p_k \in Q_k$.})] ~
    Applying fact F1, execution $\run$ is indistinguishable from $\run''=\ldots
    U_j \ldots s_{k} U_l U_k \ldots$. Then applying fact F2, $\run$ is
    indistinguishable from execution $\run'=\ldots U_j \ldots s_{k} U_k U_l \ldots$.
  \item[(\textsc{Case $p_k \in Q_l$.})]~
    With a similar reasoning, we obtain that $\run$ is indistinguishable from
    $\run'=\ldots U_j \ldots U_k U_l s_k \ldots$.
  \item[(\textsc{Case $p_k \notin Q_l \union Q_k$.})]~
    This case reduces to any of the two above cases.
  \end{compactitem}
  Note $h'$ the history $\mathfrak{F}(\run')$.
  In history $\run'$, 
  both $w_k(x_k) <_{h'} w_l(y_l)$ and $x_j \versionOrder_{h'} x_k$ hold.
  Besides, operations  $r_i(x_j)$, $r_i(y_l)$ and $w_k(x_k)$ all belong to $h'$.
  Thus, history $h'$ does not belong to \SCONSb, or transaction $T_a$ does not commit in $h'$.
  Since $\run'$ is indistinguishable from $\run$, history $h'$ is admissible.
  It follows that $T_a$ does not commit in $h'$.
  (The case $k>l$ follows a symmetrical reasoning to the case $l>k$ we considered previously.)
\end{IEEEproof}

\newtheorem*{theosconsb}{\reftheo{imp:2}}
\begin{theosconsb}
  No asynchronous failure-free \GPR system implements \SCONSb.
\end{theosconsb}

\begin{IEEEproof}
  Consider some read-only transaction $T_a$, 
  two distinct objects $x$ and $y$ read by $T_a$,
  and assume that $\replicaSetOf{x}$ and $\replicaSetOf{y}$  are disjoint.

  We reason by contradiction,
  exhibiting an admissible execution during which transaction $T_a$ never terminates.
  This execution is constructed as follows:

  \paragraph{Construction.}
  Let $\mathcal{P}$ be an initially empty FIFO list, and consider an initially null execution $\run$.
  Start executing $T_a$ by \coordOf{T_a}.
  Repeat for all $i \geq 1$.
  Add to $\mathcal{P}$ (in some arbitrary order) 
  the processes that have to execute a step for $T_a$.
  Pop from $\mathcal{P}$ the next process $p$ to execute a step for $T_a$.
  Extend $\run$ with step $s_i$, the next step of $p$.
  Let $T_i$ be an update of $x$, if $i$ is even, and $y$ otherwise.
  Start the execution of transaction $T_i$.
  Since 
  no transaction are concurrent, 
  updates are obstruction-free
  and the system is genuine, 
  there exists an extension $\run' = \run \cseqAppend U_i$ during which $T_i$ commits
  and such that in $U_i$, 
  only processes in \replicaSetOf{x}, if $i$ is odd, or in \replicaSetOf{y} otherwise, execute steps.
  Assign to $\run$ the value of $\run'$.

  By construction, execution $\run$ is flippable.
  Hence, \reflem{imp:2} tells us that transaction $T_a$ does not terminate in this run.
  Since every process in $\mathcal{P}$ eventually make a step in $\run$, $\run$ is fair.
  Because there is no synchrony assumptions, this execution is admissible.
  In \run, transaction $T_a$ never commits.
  Contradiction.
\end{IEEEproof}

\bigskip
\noindent
Our last impossibility result circumvents the cost of \SCONSa.

\newtheorem*{theosconsa}{\reftheo{imp:3}}
\begin{theosconsa}
  No asynchronous failure-free \GPR system implements \SCONSa.
\end{theosconsa}

\begin{IEEEproof}
  Consider two distinct objects $x$ and $y$ such that $\replicaSetOf{x}$ and $\replicaSetOf{y}$ are disjoint.
  Let $T_1$ be an update transaction accessing $x$, 
  $T_2$ be an update on $y$,
  and $T_a$ be a read-only transaction accessing both objects.
  
  Since updates are obstruction-free, history $h_1=r_1(x_0).w_1(x_1).c_1$ is admissible.
  Let $U_1$ be a sequence of steps such that $\refMapOf{U_1}=r_1(x_0).w_1(x_1).c_1$.

  The system \procSet satisfies non-trivial \SI.
  Consequently, there exists an extension $U_1.U_a$ of $U_1$ such that $\refMapOf{U_a}=r_a(x_1)$, 
  and history $h_2=h_1.\refMapOf{U_a}$ is admissible.

  Then, since the system supports obstruction-free updates,
  there exists an extension $U_1.U_a.U_2$ such that 
  $\refMapOf{U_2}=r_2(y_0).w_2(y_2)$, and history $h_3=h_2.\refMapOf{U_2}$ is admissible.

  Finally, we may extend $U_1.U_a.U_2$ by a sequence of steps $V_a$ such that 
  $\refMapOf{V_a}=r_a(y_2).c_2$, and $h_3.\refMapOf{V_a}$ is admissible.
  Such an extension is possible 
  since \procSet satisfies both non-trivial SI and wait-free queries.
  
  Consider the execution $U_1.U_a.U_2$.
  Applying \reflem{imp:1}, 
  only processes in \replicaSetOf{x} make steps to execute $T_a$ in this execution.
  Since \replicaSetOf{x} and \replicaSetOf{y} are disjoint, 
  it follows that $U_1.U_a.U_2$ is indistinguishable from $U_1.U_2.U_a$.
  As a consequence, the execution $U_1.U_2.U_a.V_a$ is admissible.
  Notice that $\refMapOf{U_1.U_2.U_a.V_a}$ equals 
  $r_1(x_0).w_1(x_1).c_1.r_a(x_1).r_2(y_0).w_2(y_2).r_a(y_2).c_2$.
  This history is not in \SCONSa.
  Contradiction.
\end{IEEEproof}

% \newpage
% \input{appendix/phenomena}
% \newpage
% \input{appendix/correctness_vectors}
% \newpage
% \input{appendix/correctness_jessy}
% 
